# Supplementary material for: iBatch: Saving Ethereum Fees via Secure and Cost-Effective Batching of Smart-Contract Invocations
Source: arXiv:2106.08554 source file (2021-08-24)
Supplement: Supplementary file 2 [file techrep_appendix.tex]

%Which function(s) to rewrite is application-specific. We will describe two common DApps, that is, ERC20 token contracts and decentralized exchange (DEX).
