# Supplementary material for: iBatch: Saving Ethereum Fees via Secure and Cost-Effective Batching of Smart-Contract Invocations
Source: arXiv:2106.08554 source file (2021-08-24)
Supplement: Supplementary file 3 [file wellformated_appendix.tex]

\vspace{0.2in}
\section*{Appendices}

\setcounter{section}{0}
{
%\color{red}
}

\clearpage
