# Supplementary material for: iBatch: Saving Ethereum Fees via Secure and Cost-Effective Batching of Smart-Contract Invocations
Source: arXiv:2106.08554 source file (2021-08-24)
Supplement: Supplementary file 4 [file appendix.tex]

\input{text/3_customize.tex}

\section{Detailed Security Analysis of Basic Batching Mechanism}
\label{sec:security}

Recall that in the EtherBatch's trust model, all smart contracts are trusted in the properties described in \S~\ref{sec:trustmodel}. Each user is also trusted to protect her secret key, that is, no key loss or stealing. In this trust model, we consider two types of threats for security analysis: A malicious \texttt{Batcher} service who can forge, replay, omit contract calls in the batching workflow, and a malicious user who wants to impersonate another victim user to spend her deposit. We don't consider the collusion between a \texttt{Batcher} service and a caller EOA because in practice they are in different domains.

To simplify the security analysis, we consider each secret key is locally managed by its EOA client and is not stored on the \texttt{Batcher} service. 

{\bf Malicious \texttt{Batcher} (A1)}: In this threat model, the malicious \texttt{Batcher} wants to forge a contract call from an existing user, say Alice, and include it in the batched transaction (Attack A1a). Here, Alice does not sign the contract call. To make the forged call validated (see Line 10 in Listing~\ref{lst:dispatch}), the \texttt{Batcher} has to forge the signature verifiable by Alice's public key, yet without knowing Alice's secret key. This is hard with the standard cryptography assumptions (e.g., the hardness of discrete log problem for ECDSA signature algorithms used in Ethereum).

The \texttt{Batcher} can create a Sybil account (i.e., creating a public key and private key) by itself and include in the batched transaction a contract call issued from the Sybil account. However, by doing this, it will not affect other accounts and their application-contract states.

The \texttt{Batcher} can also replay an existing contract call and include it into the batch more than once (Attack A1b). For instance, in token contacts, the \texttt{Batcher} may want to replay a \texttt{transfer()} call to double-spend tokens. Mechanically, to mount the attack, each contract call, as issued by the web3 library, is identified by its caller EOA and a distinct nonce. The contract call of the same EOA and nonce is included into one or multiple batched transactions, by a replaying \texttt{Batcher}. Based on the \texttt{Dispatcher} contract, each nonce value can only be used for once. Thus, the second time it is used by a replayed message, the \texttt{Dispatcher} contract will not forward the request.

The \texttt{Batcher} can omit a valid contract call and exclude it in any batched transaction (Attack A1c). This is a form of denial of service attack on the \texttt{Batcher} availability. Had this attack been mounted, the \texttt{Batcher} would have lost the chance to collect the batching fee from the omitted call. Thus, a rational \texttt{Batcher} would not mount the call-omission attack.

{\bf Malicious users (A2)}: In this threat model, a malicious user wants to steal another user's digital asset by exploiting the attack surface exposed by a \texttt{Dispatcher} contract and the application contract. Suppose the malicious EOA $M$ wants to impersonate a victim EOA $A$ and be able to spend her digital assets stored in the application contract. The malicious EOA may attempt to forge a call to \texttt{dispatch()} or send a fake request with the forged signature of victim $A$ to the \texttt{Batcher}. Because function \texttt{dispatch()} authenticates its caller by the \texttt{Batcher} service's signature, a malicious EOA cannot forge the \texttt{Batcher}'s signature (assume there is no collusion). Also, malicious EOA $M$ cannot forge victim $ A$'s signature, and she cannot send a forged request impersonating $A$.



\section{Earlier Measurement Results}

\begin{figure*}
\centering
  \subfloat[Batch sizes in 8-month BNB trace]{
\includegraphics[width=0.5\textwidth]{figures/BNB_yibo/exp-Numberofcallsperbatch-Indexofevery100batches.eps}
    \label{fig:timeline:bnb}
  } 
  \subfloat[Gas in 8-month BNB trace]{%
\includegraphics[width=0.5\textwidth]{figures/BNB_yibo/exp-Costpercall-Indexofevery100batches.eps}
    \label{fig:timeline:bnb:8month}
  }
\\
  \subfloat[Batch size in IDEX trace]{%
\includegraphics[width=0.5\textwidth]{figures/exp-Numberofcallsperblock-Relativeblockheight.eps}
    \label{fig:timeline:idex}
  }
  \subfloat[Gas in IDEX trace]{%
%    \includegraphics[width=0.5\textwidth]{figures/exp-Gaspertradecall-Blocknumber.eps} 
     \includegraphics[width=0.5\textwidth]{figures/exp-Gaspertradecall-Relativeblockheight.eps}
    \label{fig:eval:idex}
  }
%Gas under a 4-hour call trace of BNB token (time window: 180 second)} 
\caption{Gas cost under the traces of BNB token and IDEX}
\end{figure*}

\subsubsection{Cost in the IDEX Trace}

In this experiment, we select a sub-trace containing 198 blocks and $999$ \texttt{trade} calls which last for 50 minutes on June, 5, 2018. Figure~\ref{fig:timeline:idex} shows the distribution of batch size over time, where the number of transactions per block can be as high as 47 per block.  We replay the selected trace to the experiment platform, with and without EtherBatch. When running with EtherBatch, we use two settings of the time window, respectively to batch calls in one block and five blocks. 
Figure~\ref{fig:eval:idex} illustrates the Gas per \texttt{trade} with different block heights in the trace. Note the Gas includes both the transaction fee and contract-execution cost. The  per-invocation Gas cost varies over time/blocks because the number of calls in a batch varies. On average, EtherBatch with five blocks and one block respectively save the total Gas by  $10.1\%$ and $11.2\%$ compared with the unbatched baseline. 



\section{Additional Evaluation with EtherDelta}
\label{sec:cost:etherdelta}

\begin{figure}[!bthp]
\centering
\includegraphics[width=0.35\textwidth]{figures/etherdelta/etherdelta-exp-Gasperinvocation-Relativeblockheight.eps}
\caption{Gas under EtherDelta}
\label{fig:eval:etherdelta}
\end{figure}

\begin{table}[!htbp] %force in current page, disable float.
\caption{Average Gas per \texttt{trade} in the EtherDelta trace} 
\label{tab:avggas:etherdelta}\centering{\small
\begin{tabularx}{0.4\textwidth}{ |X|c|c|c| }
\hline
EtherBatch batch size (\# of blocks) & Total Gas (X1M) & Saving ratio
\\ \hline
1 & 279.9 & -0.23\%  
\\ \hline
2 & 272.9 & -2.71\%
\\ \hline
5 & 260.4 & -7.17\%
\\ \hline
10 & 255.4 & -8.95\%
\\ \hline
20 & 254.5 & -9.26\%
\\ \hline
0 (Unbatched B0) & 280.5  & 0
\\ \hline
\end{tabularx}
}
\end{table}

We evaluate EtherBatch's Gas under an EtherDelta trace in a similar way with that under the IDEX trace. The trace contains 1000 blocks and 2992 trade calls. The average Gas per trade call is presented in Figure~\ref{fig:eval:etherdelta}, and Table~\ref{tab:avggas:etherdelta} shows the average Gas saving of EtherBatch compared with unbatched baseline, under the varying number of blocks in a batch. The cost saving is less significant than in IDEX, which we suspect is due to the more complex smart contract in EtherDelta and lower weigh of a transaction fee. 



\section{Cost Evaluation under smaller BNB}
\begin{figure*}
\centering
  \subfloat[Batch size in BNB trace]{
    \includegraphics[width=0.25\textwidth]{figures/exp-Numberofcallsperbatch-Relativeblockheight.eps}
    \label{fig:timeline:trace}
  }
  \subfloat[Gas in BNB trace (EB is EtherBatch)]{%
    \includegraphics[width=0.25\textwidth]{figures/exp-Gaspertransfercall-Relativeblockheight.eps}
%exp-Timeline-24hours-4hours-period.eps}
    %\includegraphics[width=0.4\textwidth]{figures/exp-Timeline.eps}
    \label{fig:timeline:4h}
  }
  \subfloat[Batch size in IDEX trace]{%
     \includegraphics[width=0.25\textwidth]{figures/exp-Numberofcallsperblock-Relativeblockheight.eps}
    \label{fig:timeline:idex}
  }
  \subfloat[Gas in IDEX trace]{%
%    \includegraphics[width=0.25\textwidth]{figures/exp-Gaspertradecall-Blocknumber.eps}
     \includegraphics[width=0.25\textwidth]{figures/exp-Gaspertradecall-Relativeblockheight.eps}
    \label{fig:eval:idex}
  }
%Gas under a 4-hour call trace of BNB token (time window: 180 second)}
\caption{Gas under the traces of BNB token and IDEX}
\end{figure*}

In this subsection, we present the Gas evaluation of EtherBatch using real workloads collected from Ethereum mainnet. Here we consider the two applications in our case study, namely IDEX and BNB tokens.

\vspace{-0.1in}
\subsubsection{Trace Collection \& Experiment Setup}

We run an instrumented \texttt{Geth} node and synchronize it with the Ethereum mainnet. During the (basic) node synchronization, the instrumented node intercepts all the transactions and internal calls, and dump them to local log storage; from there, we extract and reconstruct the function calls to ERC20 token contracts. We use the traces for two popular cases: the BNB token (or Binance~\cite{me:Binance}) and the IDEX exchange DApp.

To prepare the trace for experiments, we replace the addresses (or public keys) in the trace by new public keys generated under our control. This allows us to know the secret key of the addresses in the trace and to make it possible to replay the trace for experiments. During the experiments, we replay the trace based on the block timestamps and drive it into the EtherBatch. While we replay both internal and external calls, we apply EtherBatch only to the external calls in the trace.

\vspace{-0.1in}
\subsubsection{Cost in the BNB Trace}

The BNB trace we selected for evaluation is a four-hour collection of transactions sent to the BNB smart contract. The trace particularly includes a section of ``flash'' transactions, as shown in Figure~\ref{fig:timeline:trace} (will be described), that are issued intensively in a one-hour period to clear BNB accounts; specifically, these transactions transfer tokens from different senders' accounts to a single receiver account and clear the sender's accounts (by resetting balance to zero). The Gas of these calls are typically negative because of the clear-storage operations.

We use the time window of $180$ seconds, that is, all invocations falling under the same $180$ seconds may be put in a batch. When applying this batching window to the BNB trace, it results in batches with varying sizes illustrated as in Figure~\ref{fig:timeline:trace}. Most $180$-second batches have more than 10 invocations. Between $0.5$-th and $1.5$-th hours, there are flash transactions. On top of this, we enforce the minimal batching policy with $N_{min}=5$. That is, the time windows with fewer than $5$ invocations will not result in batched transactions; instead, the invocations are sent in dedicated, unbatched transactions (B0).

The Gas cost of the four-hour trace is illustrated in Figure~\ref{fig:timeline:4h}. In general, the two EtherBatch variants result in lower Gas per invocation during any time point of this trace. Particularly, between $0.5$-th and $1.5$-th hour, the saving of EtherBatch is the most significant because the intensive flash transactions enables effective amortization of translation fees by EtherBatch. 
%Besides, the unbatched baseline's Gas per invocation varies because the \texttt{transfer()} may insert or update an account's balance, depending on whether it is the first time to do so (recall the different costs of updating and inserting a word in Table~\ref{tab:costmodel}).

\begin{table}[!htbp] %force in current page, disable float.
\caption{Average cost per invocation}
\label{tab:avggas}\centering{\small
\begin{tabularx}{0.4\textwidth}{ |X|c| }
  \hline
  \multirow{2}{*}{Approaches} & Average cost per  \\ 
  & invocation (10K Gas) \\ \hline
EtherBatch & $1.64$ ($-29.3\%$)\\ \hline
EtherBatch-inlined & $1.56$ ($-32.7\%$)\\ \hline
Batched baseline (B1) & $2.23$ ($-3.88\%$)\\ \hline
Unbatched baseline (B0) & $2.32$\\ \hline
\end{tabularx}
}
\end{table}

Overall, the average Gas per invocation during these four hours is presented in Table~\ref{tab:avggas}; here, EtherBatch save Gas by up to $32.7\%$ compared with unbatched baseline B0.




\section{System Integration: Design Rationale}
\label{sec:baseline}

The EtherBatch requires \texttt{Dispatcher} sending internal calls to a callee smart contract. In our strawman design, the \texttt{Dispatcher} sends internal calls to unmodified callee smart contracts. However, an unmodified callee contract only accepts invocations whose \texttt{msg.sender} is the original caller EOA. In our case, the msg.sender of an internal call changes to the contract account of \texttt{Dispatcher} itself. Naively sending the internal calls to unmodified callee contracts would fail.

Ideally, one may want to restrain from modifying callee smart contracts. We have explored the design space without success. For instance, in the case that the callee is an ERC20 token, one can piggyback the \texttt{approve}/\texttt{transferFrom} workflow to enable the internal calls. That is, when the \texttt{Dispatcher} wants to \texttt{transfer} a token from account A to B, it  issues an internal call to \texttt{transferFrom} its allowance to B, assuming the allowance is \texttt{approve}'ed by A. 
We call this design by Baseline Batching (B1).
While B1 does not fail the internal call, it causes overhead - The need to send an additional transaction to call \texttt{approve} and to update the storage of allowance incur additional costs that would outweigh the saving by batching, as examined in our implementation of B1. A more detailed analysis of B1's cost is presented in Appendix~\ref{sec:costanalysis}. 

Alternatively, one may let the \texttt{Dispatcher} use the \texttt{delegatecall} to invoke the callee contract. A \texttt{delegatecall} inclines the code being called (the callee code) in the execution context of a caller. Unfortunately, the design does not work either, because the sender of the batched transaction is not the original caller EOA.

The above experience motivates our design choice to rewrite the DApp's callee smart contract to work with \texttt{Dispatcher} at minimal costs.


\section{Service Profitability}
\label{sec:pricing}

An EtherBatch user needs to pay for the service. Briefly, a user registers her public key in the service and make an Ether payment to the EOA controlled by the EtherBatch (e.g., $D$). The EtherBatch will only batch the invocation requests from the registered public keys which have paid. Making EtherBatch a paid service is necessary to prevent malicious users from depleting EtherBatch's account. 

A naive design for EtherBatch service charge is that the \texttt{Dispatcher} contract receives the initial payment to register a public key and does the accounting for individual invocations. More concretely, the \texttt{Dispatcher} contract maintains a list of registered public keys and, upon each invocation of public key $K$, decrements the budget associated with $K$. While inheriting the blockchain security, this on-chain design of accounting incurs high cost.

In EtherBatch's design, we propose to place accounting on the off-chain \texttt{Batcher} service. The \texttt{Batcher} server, once observing the finality of a payment transaction from EOA $K$ to EOA $D$, registers the public key $K$ locally. The server then conducts the accounting upon individual invocation requests. For each invocation from $K$, the server deduces certain points from $ K$'s balance stored locally. 

%{\bf Security analysis and hardening}: In the above design, the \texttt{Batcher} server is incentivized not to process the invocations from unregistered EOAs, thus preventing such EOAs mounting DOS attacks to deplete \texttt{Batcher} 's Ether.
%However, the \texttt{Batcher} server may be malicious and greedy such that it refuses to process the invocation requests from paid EOAs. To prevent this attack, the \texttt{Dispatcher} contract serves as an escrow and has a \texttt{disputeResolve()} function. %The dispute resolution subprotocol work as following: YYY.

{\bf Service pricing and profitability analysis}: In the initial payment, the user purchases the EtherBatch service to batch $U$ contract calls (within a certain time period) at the price of $V$ Ethers. 

In order for the user to save money, it entails the following, which means the Ether she spends on using EtherBatch should be less than the Ether without EtherBatch.

{\small
\begin{eqnarray}
\nonumber
&&
\frac{V}{gasPrice}+21000<(21000+2175X)*U
\\\nonumber
&\Rightarrow&
\frac{V}{gasPrice}<(21000+2175X)*U-21000\defeq{}V_{max}(U)
\end{eqnarray}
}

In order for the \texttt{Batcher} service to be profitable, it entails the following: 

{\small
\begin{eqnarray}
\nonumber
&&
[21000\frac{1}{N}+10053+4352X]*U<\frac{V}{gasPrice}
\\\nonumber
&\Rightarrow&
\frac{V}{gasPrice}>[21000\frac{1}{N}+10053+4352X]*U\defeq{}V_{min}(U)
\end{eqnarray}
}

{\scriptsize
\begin{eqnarray}
\nonumber
&&V_{min}(U)<V_{max}(U)
\\\nonumber
&\Rightarrow&[21000\frac{1}{N}+10053+4352X]*U<(21000+2175X)*U-21000
\\\nonumber
&\Rightarrow&U>21000/[21000(1-\frac{1}{N})-2177X-10053]\defeq{}U_{min}
\end{eqnarray}
}

In summary, for the profitability of EtherBatch and \texttt{Batcher} service, each user should purchase at least $U_{min}$ batched invocations.

\section{Design of Batching Baseline (B1)}
\label{sec:baseline:details}

Recall that our system model consists of EOAs managed on the client-side, an RPC service running the batcher component, a dispatcher smart contract and application smart contracts. The baseline protocol runs with a similar initial state with EtherBatch described in \S~\ref{sec:etherbatch}. Here, we describe the details of the basic protocol.

Now consider a specific EOA's application-contract call in a batch of $N-1$ other contract calls (potentially from other EOAs). The contract call is identified by five parameters, $call_i = \langle{}contract, function, args, PK_i, sig\rangle{}$. That is, the call is to invoke application contract $contract$'s function $func$ with arguments $args$. The contract call is signed by EOA $PK_i$'s secret key such that the produced signature $sig$ can be verified by the blockchain using public key $PK_i$.
In practice, these call parameters can be obtained by intercepting the javascript/web3 calls on the client-side, which is described in \S~\ref{sec:impl}.

The RPC batcher service receives multiple calls, $call_i, \forall{i}\in{[1,N]}$, from different EOAs $PK_i$. It batches them into one Etheurem transaction, leveraging the ``\texttt{data}'' field in the Ethereum transaction model. Specifically, the batched transaction is sent from the EOA of batcher service and is bound for the dispatcher smart contract, to invoke the \texttt{dispatch()} function. The function arguments are the concatenation of all application-contract calls $call_1\|\cdots{}call_N$. The generation of the batched transaction is illustrated in Equations~\ref{eqn:batchtx:baseline}.

{\scriptsize
\begin{eqnarray}
\forall{i}, call_i &=&\langle{}contract_i, function_i, args_i, PK_i, sig_i\rangle{} 
\label{eqn:batchtx:baseline}
\\ \nonumber
args &=& call_1 \| call_2 \|\dots\| call_N \\ \nonumber
data &=& \langle{}contract:dispatcher, function:dispatch, args:args\rangle{}  \\ \nonumber
batchtx &=& from:PK_{batcher}, to:PK_{dispatcher}, sig_{SK_{batcher}}, value, data  
\end{eqnarray}
}

The dispatcher smart contract receives the batched transaction $batchtx$ and runs the \texttt{dispatch()} function. This function parses the batched transaction and extracts individual application calls (i.e., $call_i$). For each call, it then verifies the signature against the provided EOA's public key $\texttt{erecover}_{PK_i}(call_i, sig_i)$. If it passes, the dispatcher contract would issue an internal call bound for the application contract, that is, $cntr\_app_i.function_i(args_i)$. The pseudo-code of the dispatcher function is illustrated in Figure~\ref{lst:dispatch}. Note that the verification function supported in Solidity is $\texttt{erecover}()$. 

\section{Additional Evaluation}

\subsection{IDEX Workload}
\label{appdx:idex:overalltrace}
\begin{figure}[!bthp]
\centering
%\includegraphics[width=0.485\textwidth]{figures/mapping300block-start0.eps}
\includegraphics[width=0.485\textwidth]{figures/mapping300block-new.eps}
\caption{The distribution of four function invocations in \texttt{IDEX1} over relative block height. (The first block, or the beginning of the trace, occurs on Sep. 27, 2017).}
\label{fig:workload:idex}
\end{figure}

{\bf Understand the workload}:
We study a trace collected from Ethereum transaction history. The trace contains all transactions that invoke a function in the \texttt{IDEX1} smart contract from Sep. 27, 2017 to Feb 23, 2019. There are about $5.87$ million such transactions, where function \texttt{trade} accounts for $55.6\%$ of the transactions, \texttt{adminWithdraw} accounts for $20.5\%$,
\texttt{deposit} accounts for $12.5\%$, and
\texttt{depositToken} accounts for $11.4\%$. The distribution of different transactions over time (or the relative height of every $300$ blocks) is plotted in Figure~\ref{fig:workload:idex}. The highest value in the figure suggests that there are $2784$ invocations in continuous $300$ blocks, which makes $9$ transactions per block on average.

\section{Alternative Design: Off-chain Audit-based Protocol}
The protocol supports the general-case batching, that is, batching Type S4 invocations.  
Initially, suppose there are $N$ invocations and the $i$-th invocation is represented in the following format: the caller's address/public key \texttt{EOA$_i$}, the nonce \texttt{nonce$_i$}, callee smart contract address \texttt{cntr$_i$}, function name \texttt{func$_i$}, argument list \texttt{args$_i$}, and caller's signature \texttt{sig$_i$} (in Equation~\ref{eqn:appdx:1:invocation}).

Given this initial state, the batching protocol works in four steps:
1) The \texttt{Batcher} batches all invocations in a transaction, signs it using \texttt{Batcher}'s private key and makes it received by smart contract \texttt{Dispatcher}'s \texttt{dispatch} function. This is presented in Equation~\ref{eqn:appdx:2:batch} where \texttt{CA} is the address of smart contract \texttt{Dispatcher}.

\vspace{-0.1in}
{\scriptsize
\begin{eqnarray}
\forall{i},  \texttt{call}_i &=&\langle{}  \texttt{EOA}_i,  \texttt{nonce}_i, \texttt{cntr}_i,  \texttt{func}_i,  \texttt{args}_i, \texttt{sig}_i\rangle{}
\label{eqn:appdx:batchtx}
\label{eqn:appdx:1:invocation}
\\ \nonumber
 \texttt{dispatch\_args} &=&  \texttt{call}_1 \|  \texttt{call}_2 \|\dots\|  \texttt{call}_N \\ \nonumber
 \texttt{data} &=& \langle{}\texttt{dispatch\_func},  \texttt{dispatch\_args}\rangle{}  \\ \nonumber
 \texttt{tx} &=& \langle{} \texttt{EOA}_{\texttt{Batcher}}, \texttt{nonce}_{\texttt{Batcher}}, \texttt{CA}_{\texttt{Dispatcher}}, \\
&& \texttt{sig}_{{\texttt{Batcher}}}, \texttt{value}, \texttt{data}\rangle{}
\label{eqn:appdx:2:batch}
\end{eqnarray}
}
\vspace{-0.1in}

On the blockchain, 2) in function \texttt{dispatch\_func}, smart contract \texttt{Dispatcher} parses the transaction and extract the original invocations \texttt{call$_i$} before forwarding them to callees, namely \texttt{cntr$_i$} and \texttt{func$_i$}.
The pseudo code of \texttt{Dispatcher} is in Appendix~\ref{sec:code:dispatcher}. Particularly, smart contract \texttt{Dispatcher} internally verifies the signature of each extracted invocation against its caller's public key; this can be done by using Solidity function $\texttt{ecrecover}(\texttt{call}_i, \texttt{sig}_i, \texttt{EOA}_i)$. If successful, the \texttt{Dispatcher} then internal-calls the callee smart contract.

3) The callee function executes the body of the function under the given arguments \texttt{args}$_i$.

4) Waiting after the call is executed, the caller audits the Ethereum transaction history to monitor if the untrusted \texttt{Batcher} has honestly sent the caller's invocation. Specifically, the \texttt{Batcher} service returns the caller the ID of the batch transaction that includes her invocation. The caller EOA then verifies the inclusion of the batch transaction in the Ethereum history (e.g., by running an SPV client against the mainnet) and verifies the inclusion of the invocation in the transaction's data field. Optionally, the caller checks the non-existence of a replayed copy of the invocation among all batch transactions received by \texttt{Dispatcher} in the Ethereum history.

Note that each invocation is identified by a unique pair of $\langle{}\texttt{EOA}_i, \texttt{nonce}_i\rangle$ in the argument of \texttt{dispatch} function. This ID is also signed by the caller, so that each invocation can be authenticated and a malicious \texttt{Batcher} cannot use one invocation to impersonate another invocation. This is important for the security against replaying attacks.

{\bf Security analysis}: Recall that the off-chain \texttt{Batcher} can mount attacks to forge, modify, replay and omit invocation requests from a caller EOA. As \texttt{Dispatcher} verifies any invocation against its caller signature, it is hard for the \texttt{Batcher} to forge or modify the invocation.

Besides, the \texttt{Batcher} who omits an invocation cannot forge a batch transaction in the Ethereum history that includes the invocation. Alternatively, the \texttt{Batcher} may return the ID of a batch transaction in Ethereum history that does not include the invocation. Eitherway, the caller audit will fail and the invocation omission will be detected.

At last, the \texttt{Batcher} who replays an invocation has to include the replayed invocation in a batch transaction she generates. Given an invocation identified by pair $\langle{}\texttt{EOA}_{i}, \texttt{nonce}_{i}\rangle{}$, the caller \texttt{EOA}$_{i}$ can sift through the Ethereum history to find the replayed invocation with the same $\langle{}\texttt{EOA}_{i}, \texttt{nonce}_{i}\rangle{}$ pair. Note that because of the unique nonce and caller signature, the \texttt{Batcher} cannot use confuse an auditing caller that a different invocation is a replay of another invocation, even if they are of the same argument values. Also, note that the caller conducts the audits by retrieving relevant transactions directly from the Ethereum nodes in the mainnet, without going through the \texttt{Batcher}. Thus the retrieved transactions can be with integrity, under the standard assumption of the honest majority of mainnet nodes.


Once a replay/omission attack is detected, the caller can present an evidence of it to an external payout scheme (e.g., a smart contract that resolves disputes) to penalize the misbehaving \texttt{Batcher}.
